# Supplementary material for: Combinatorial geometry of neural codes, neural data analysis, and neural networks
Source: arXiv:2209.07583 source file (2022-09-15)
Supplement: Supplementary file 3 [file Dedication.tex]

% Place the dedication below.
