# Supplementary material for: Combinatorial geometry of neural codes, neural data analysis, and neural networks
Source: arXiv:2209.07583 source file (2022-09-15)
Supplement: Supplementary file 4 [file ListOfSymbols.tex]

% Place the list of symbols below.
%\begin{eqlist}[\def\makelabel#1{\hfill#1}\labelsep 1em]
%
%%\item[$\alpha$]
%%The first greek letter, p.~\pageref{ChX-figure: FigureLabel3}
%%
%
%
%\end{eqlist}
