# Supplementary material for: Combinatorial geometry of neural codes, neural data analysis, and neural networks
Source: arXiv:2209.07583 source file (2022-09-15)
Supplement: Supplementary file 6 [file UserDefinedCommands.tex]

% Place user-defined commands below.

% Define the \acro command.
\makeatletter
\newif\ifFirstPar       \FirstParfalse
\def\smc{\sc}
\def\ninepoint{\small}
\DeclareRobustCommand\SMC{%
  \ifx\@currsize\normalsize\small\else
   \ifx\@currsize\small\footnotesize\else
    \ifx\@currsize\footnotesize\scriptsize\else
     \ifx\@currsize\large\normalsize\else
      \ifx\@currsize\Large\large\else
       \ifx\@currsize\LARGE\Large\else
        \ifx\@currsize\scriptsize\tiny\else
         \ifx\@currsize\tiny\tiny\else
          \ifx\@currsize\huge\LARGE\else
           \ifx\@currsize\Huge\huge\else
            \small\SMC@unknown@warning
 \fi\fi\fi\fi\fi\fi\fi\fi\fi\fi
}
\newcommand\SMC@unknown@warning{\TBWarning{\string\SMC: unrecognised
    text font size command -- using \string\small}}
\newcommand\textSMC[1]{{\SMC #1}}
\newcommand\acro[1]{\textSMC{#1}\@}

\makeatother

% command for vectors
\newcommand{\bv}[1]{\ensuremath{\vec{#1}}}
% command for unit vectors
\newcommand{\uv}[2][blank]{%
\ifthenelse{\equal{#1}{blank}}%
{\ensuremath{\hat{u}_{#2}}}%
{}%
%
\ifthenelse{\equal{#1}{.}}%
{\ensuremath{\dot{\hat{u}}_{#2}}}%
{}%
%
\ifthenelse{\equal{#1}{'}}%
{\ensuremath{\hat{u}'_{#2}}}%
{}%
}
\newcommand{\ui}{\ensuremath{\hat{\imath}}}
\newcommand{\uj}{\ensuremath{\hat{\jmath}}}
\newcommand{\uk}{\ensuremath{\hat{k}}}
